# Supplementary material for: Unlocking Diversity of Fast-Switched Optical Data Center Networks with Unified Routing
Source: arXiv:2412.00266 source file (2024-11-29)
Supplement: Supplementary file 1 [file appendix.tex]

\appendix

\subsection{Queue state maintaining}\label{appendix:queue_state}

The queue state register serves as the cache of queue depth estimation.
When the queue depth estimation indicates the queue is full, the queue state will be updated from unfull to full by a recirculated signal packet.
In this scenario, the queue state may become outdated when the signal packet is under recirculation.
This issue can be addressed by adjusting the maximum queue depth based on the recirculation delay multiplied by the port bandwidth.
This prevents any packets from being incorrectly enqueued while slightly reducing bandwidth utilization, especially for short slice durations.
However, with shorter slice durations, the impact of incorrectly enqueued packets is mitigated due to the shorter cycle duration.
So we can set the adjusting value smaller when the slice is short to balance the tradeoff.
